# Supplementary material for: Non-Compact Atomic Insulators
Source: arXiv:2107.13556 source file (2021-11-29)
Supplement: Supplementary file 1 [file suppfigs.pdf]

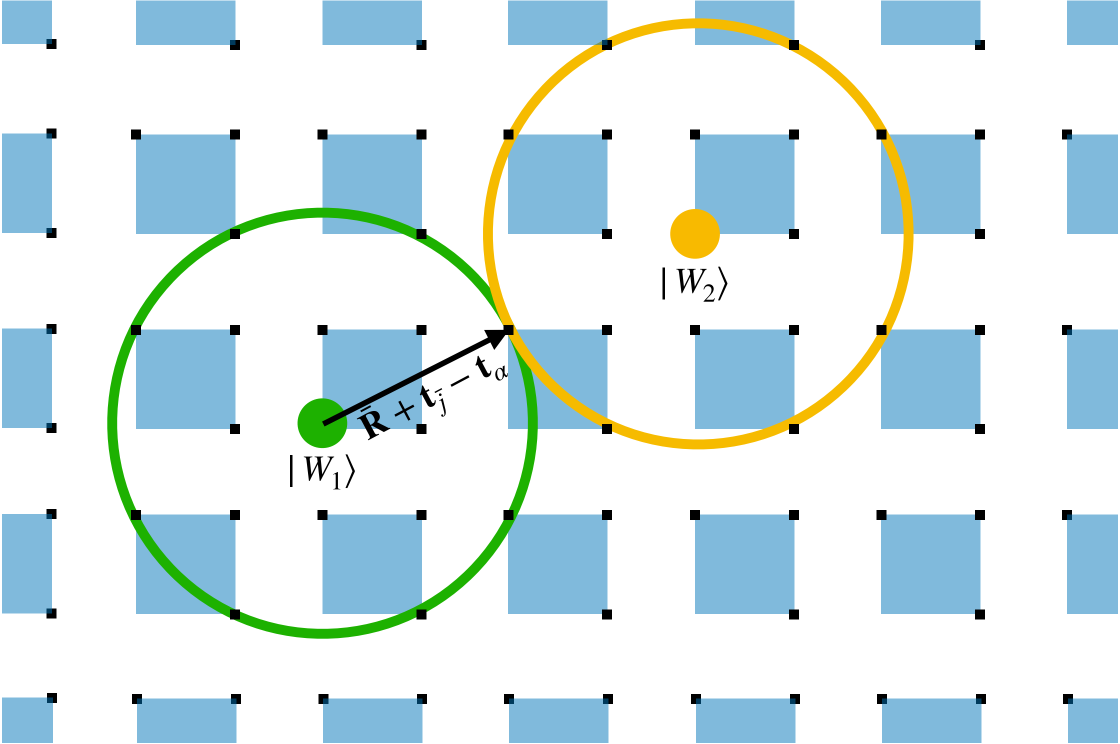
$|W_2\rangle$
$\bar{\mathbf{R}} + \mathbf{t}_j - \mathbf{t}_\alpha$
$|W_1\rangle$

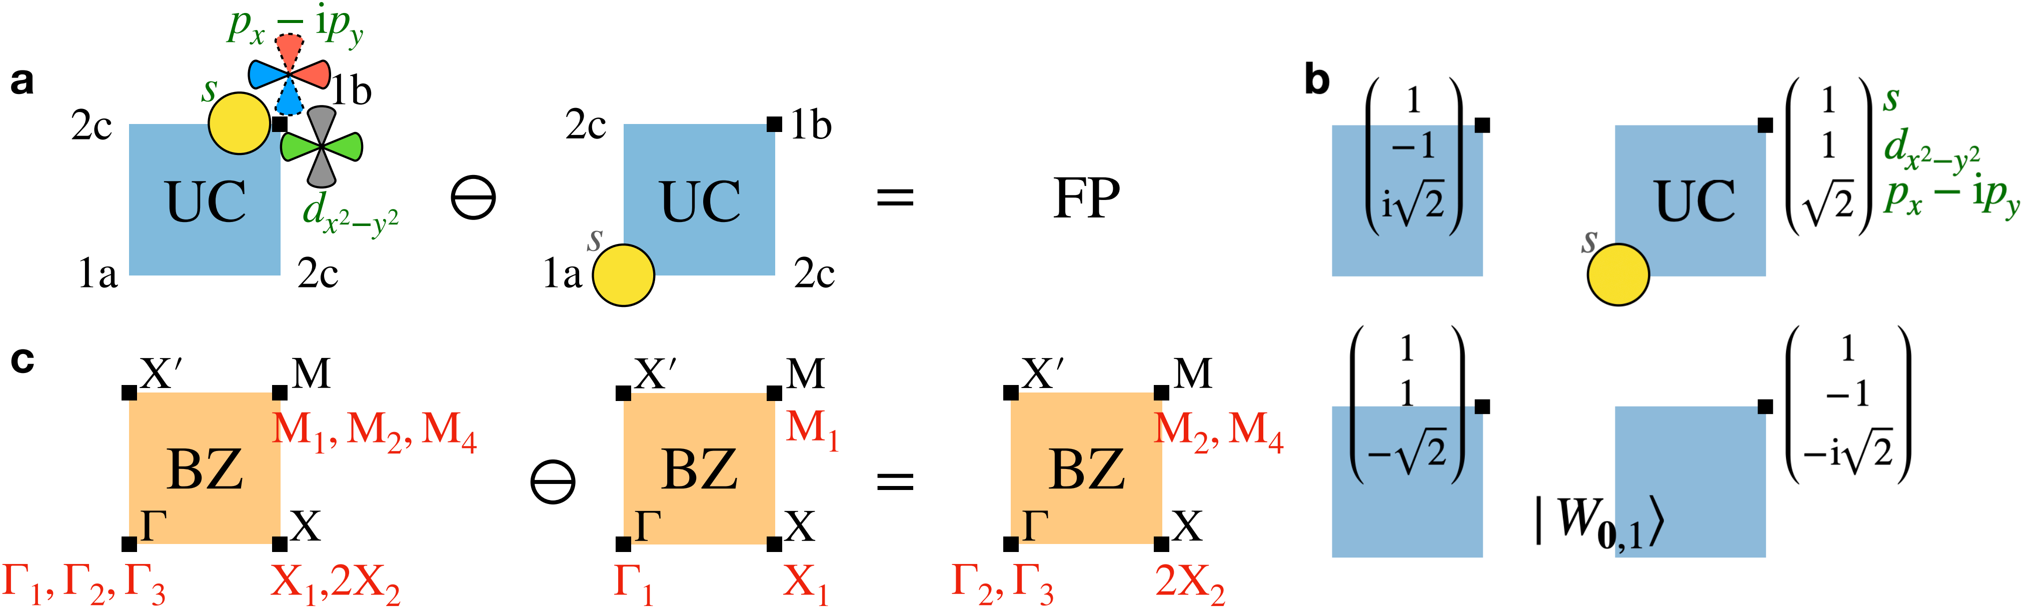

a
$p_x - ip_y$
s
1b
2c
UC
$d_{x^2-y^2}$
1a
2c
⊖
2c
1b
UC
s
1a
2c
=
FP
b
$\begin{pmatrix} 1 \\ -1 \\ i\sqrt{2} \end{pmatrix}$
$\begin{pmatrix} 1 \\ 1 \\ \sqrt{2} \end{pmatrix}$
s
$d_{x^2-y^2}$
$p_x - ip_y$
UC
s
$\begin{pmatrix} 1 \\ 1 \\ -\sqrt{2} \end{pmatrix}$
$\begin{pmatrix} 1 \\ -1 \\ -i\sqrt{2} \end{pmatrix}$
$|W_{\mathbf{0},1}\rangle$
c
X′
M
BZ
$M_1, M_2, M_4$
Γ
X
$\Gamma_1, \Gamma_2, \Gamma_3$
$X_1, 2X_2$
⊖
X′
M
BZ
$M_1$
Γ
X
$\Gamma_1$
$X_1$
=
X′
M
BZ
$M_2, M_4$
Γ
X
$\Gamma_2, \Gamma_3$
$2X_2$

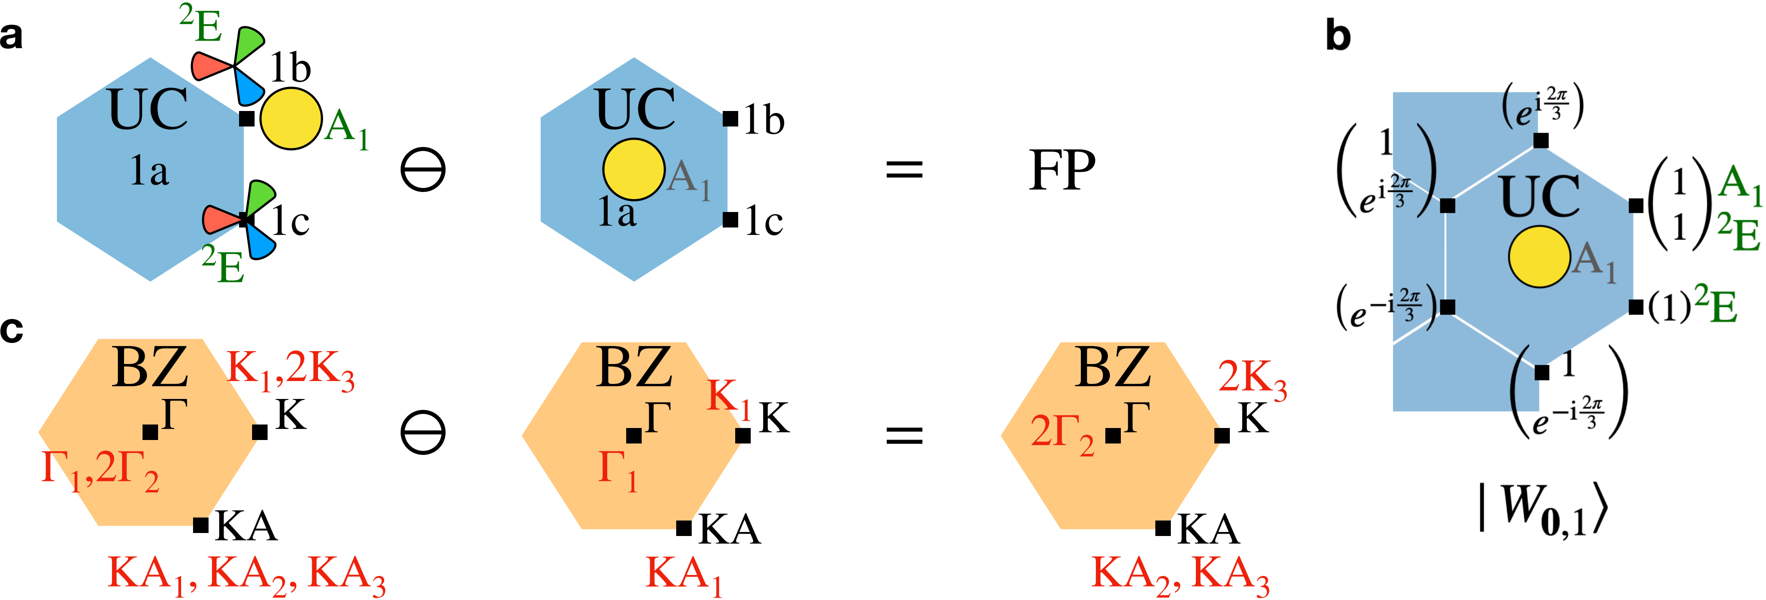

a
$^2$E
1b
UC
1a
$A_1$
1c
$^2$E
⊖
UC
1b
$A_1$
1a
1c
=
FP
b
$\left(e^{i\frac{2\pi}{3}}\right)$
$\begin{pmatrix}1\\ e^{i\frac{2\pi}{3}}\end{pmatrix}$
UC
$\begin{pmatrix}1\\ 1\end{pmatrix}$ $A_1$ $^2$E
$A_1$
$\left(e^{-i\frac{2\pi}{3}}\right)$
$(1)$ $^2$E
$\begin{pmatrix}1\\ e^{-i\frac{2\pi}{3}}\end{pmatrix}$
$|W_{\mathbf{0},1}\rangle$
c
BZ
$K_1, 2K_3$
Γ
K
$\Gamma_1, 2\Gamma_2$
KA
$KA_1, KA_2, KA_3$
⊖
BZ
$K_1$
Γ
K
$\Gamma_1$
KA
$KA_1$
=
BZ
$2K_3$
$2\Gamma_2$
Γ
K
KA
$KA_2, KA_3$

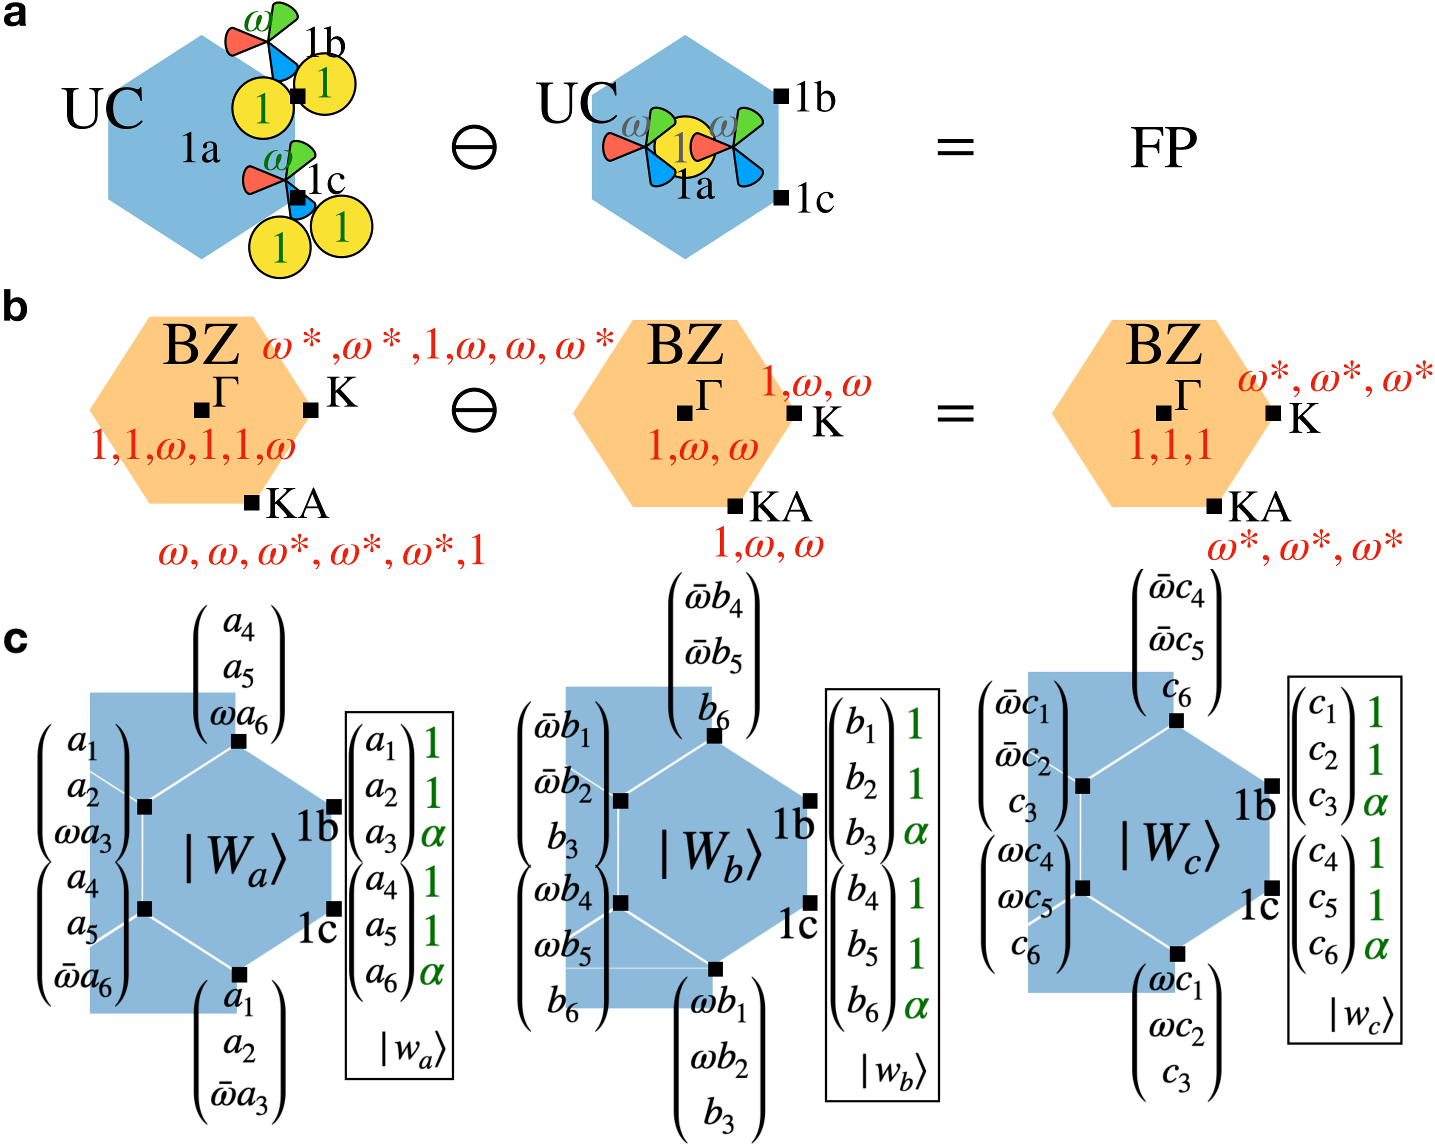
a
UC
1a
1b
1c
⊖
UC
1b
1a
1c
=
FP
b
BZ
Γ
K
KA
ω*, ω*, 1, ω, ω, ω*
1, 1, ω, 1, 1, ω
ω, ω, ω*, ω*, ω*, 1
⊖
BZ
Γ
K
KA
1, ω, ω
1, ω, ω
1, ω, ω
=
BZ
Γ
K
KA
ω*, ω*, ω*
1, 1, 1
ω*, ω*, ω*
c
|W_a⟩
1b
1c
|w_a⟩
|W_b⟩
1b
1c
|w_b⟩
|W_c⟩
1b
1c
|w_c⟩

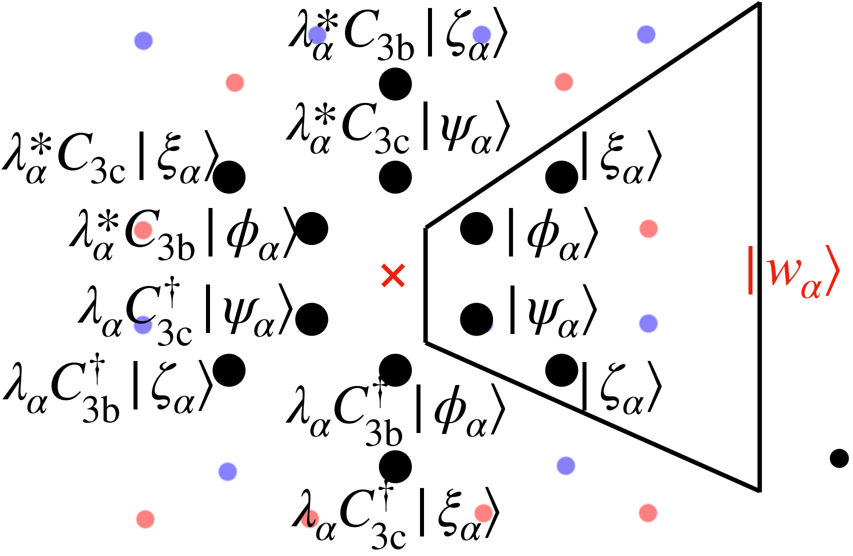


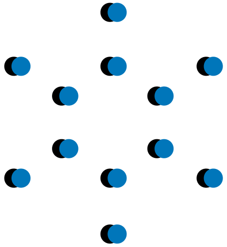

**(1)**

$$\begin{pmatrix} \langle \phi_\alpha | \\ \langle \psi_\alpha | \\ \langle \xi_\alpha | \\ \langle \zeta_\alpha | \end{pmatrix}^{\mathrm{T}} \begin{pmatrix} | \phi_\beta \rangle \\ | \psi_\beta \rangle \\ | \xi_\beta \rangle \\ | \zeta_\beta \rangle \end{pmatrix} \delta_{\lambda_\alpha \lambda_\beta} = 3\delta_{\alpha\beta}$$

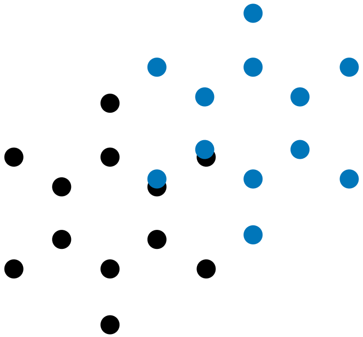

**(2)**

$$\begin{pmatrix} \langle \phi_\alpha | \\ \langle \psi_\alpha | \\ \langle \xi_\alpha | \\ \langle \zeta_\alpha | \end{pmatrix}^{\mathrm{T}} \begin{pmatrix} 0 & 0 & 0 & \lambda_\beta C_{3b}^\dagger \\ 0 & 0 & 0 & 0 \\ 0 & \lambda_\beta C_{3c}^\dagger & 0 & 0 \\ 0 & 0 & 0 & 0 \end{pmatrix} \begin{pmatrix} | \phi_\beta \rangle \\ | \psi_\beta \rangle \\ | \xi_\beta \rangle \\ | \zeta_\beta \rangle \end{pmatrix} = 0$$

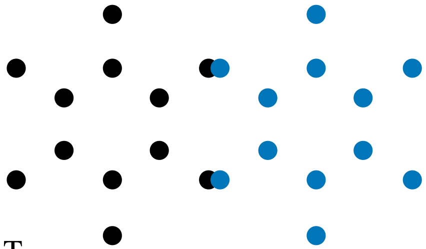

**(3)**

$$\begin{pmatrix} \langle \phi_\alpha | \\ \langle \psi_\alpha | \\ \langle \xi_\alpha | \\ \langle \zeta_\alpha | \end{pmatrix}^{\mathrm{T}} \begin{pmatrix} 0 & 0 & 0 & 0 \\ 0 & 0 & 0 & 0 \\ 0 & 0 & \lambda_\beta^* C_{3c} & 0 \\ 0 & 0 & 0 & \lambda_\beta C_{3b}^\dagger \end{pmatrix} \begin{pmatrix} | \phi_\beta \rangle \\ | \psi_\beta \rangle \\ | \xi_\beta \rangle \\ | \zeta_\beta \rangle \end{pmatrix} = 0$$

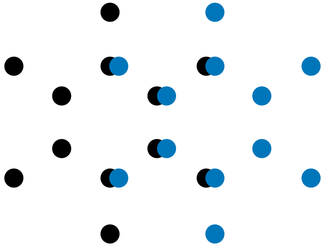

**(4)**

$$\begin{pmatrix} \langle \phi_\alpha | \\ \langle \psi_\alpha | \\ \langle \xi_\alpha | \\ \langle \zeta_\alpha | \end{pmatrix}^{\mathrm{T}} \begin{pmatrix} \lambda_\beta^* C_{3b} & 0 & 0 & \lambda_\alpha^* \lambda_\beta \\ 0 & \lambda_\beta C_{3c}^\dagger & \lambda_\alpha \lambda_\beta^* & 0 \\ 0 & \lambda_\beta^* C_{3c} & 0 & 0 \\ \lambda_\beta C_{3b}^\dagger & 0 & 0 & 0 \end{pmatrix} \begin{pmatrix} | \phi_\beta \rangle \\ | \psi_\beta \rangle \\ | \xi_\beta \rangle \\ | \zeta_\beta \rangle \end{pmatrix} = 0$$

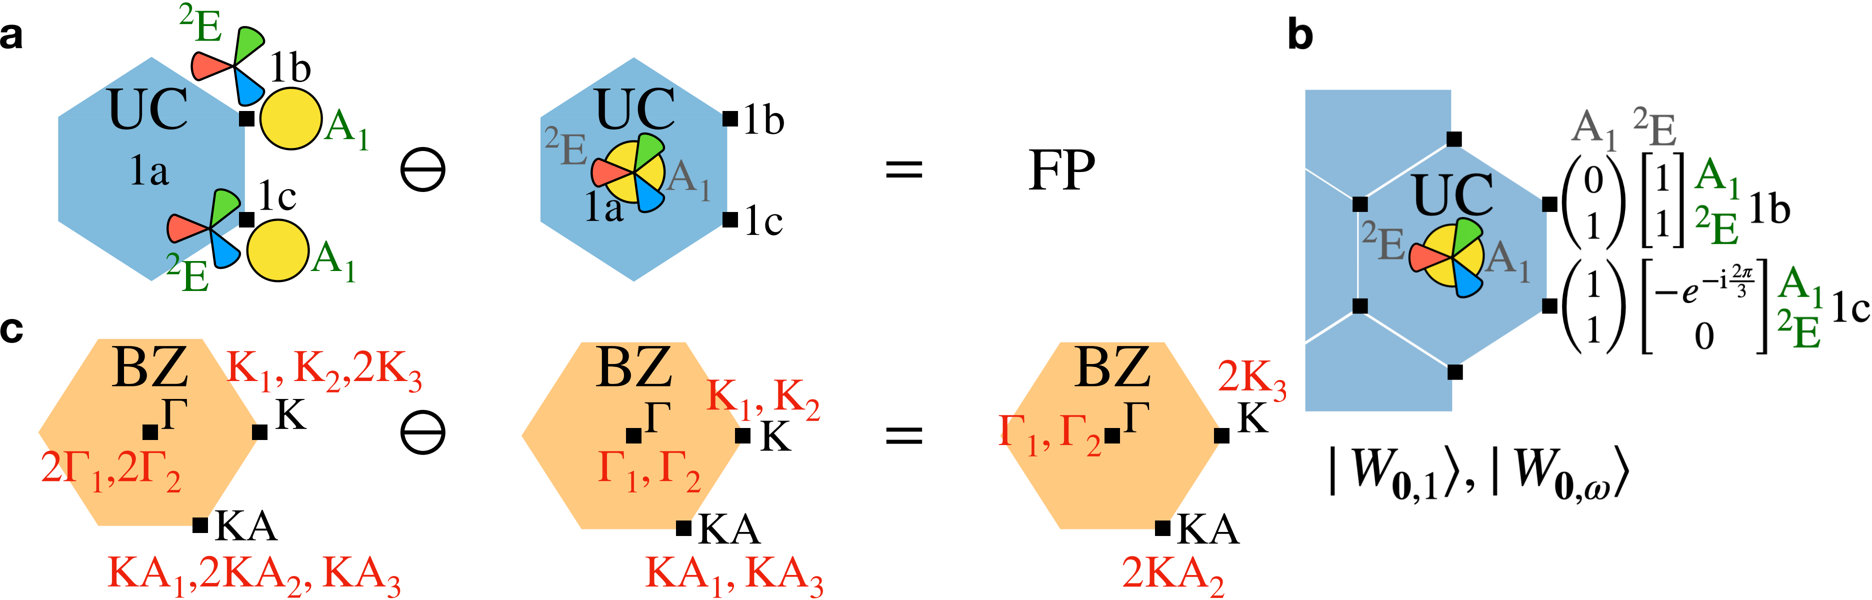

a
UC
1a
1b
1c
$^2$E
$A_1$
$\ominus$
UC
1a
1b
1c
$^2$E
$A_1$
=
FP
b
$A_1$ $^2$E
UC
$^2$E
$A_1$
$\begin{pmatrix}0\\1\end{pmatrix}$ $\begin{bmatrix}1\\1\end{bmatrix}$ $A_1$ $^2$E 1b
$\begin{pmatrix}1\\1\end{pmatrix}$ $\begin{bmatrix}-e^{-i\frac{2\pi}{3}}\\0\end{bmatrix}$ $A_1$ $^2$E 1c
$|W_{\mathbf{0},1}\rangle, |W_{\mathbf{0},\omega}\rangle$
c
BZ
Γ
K
KA
$K_1, K_2, 2K_3$
$2\Gamma_1, 2\Gamma_2$
$KA_1, 2KA_2, KA_3$
$\ominus$
BZ
Γ
K
KA
$K_1, K_2$
$\Gamma_1, \Gamma_2$
$KA_1, KA_3$
=
BZ
Γ
K
KA
$2K_3$
$\Gamma_1, \Gamma_2$
$2KA_2$

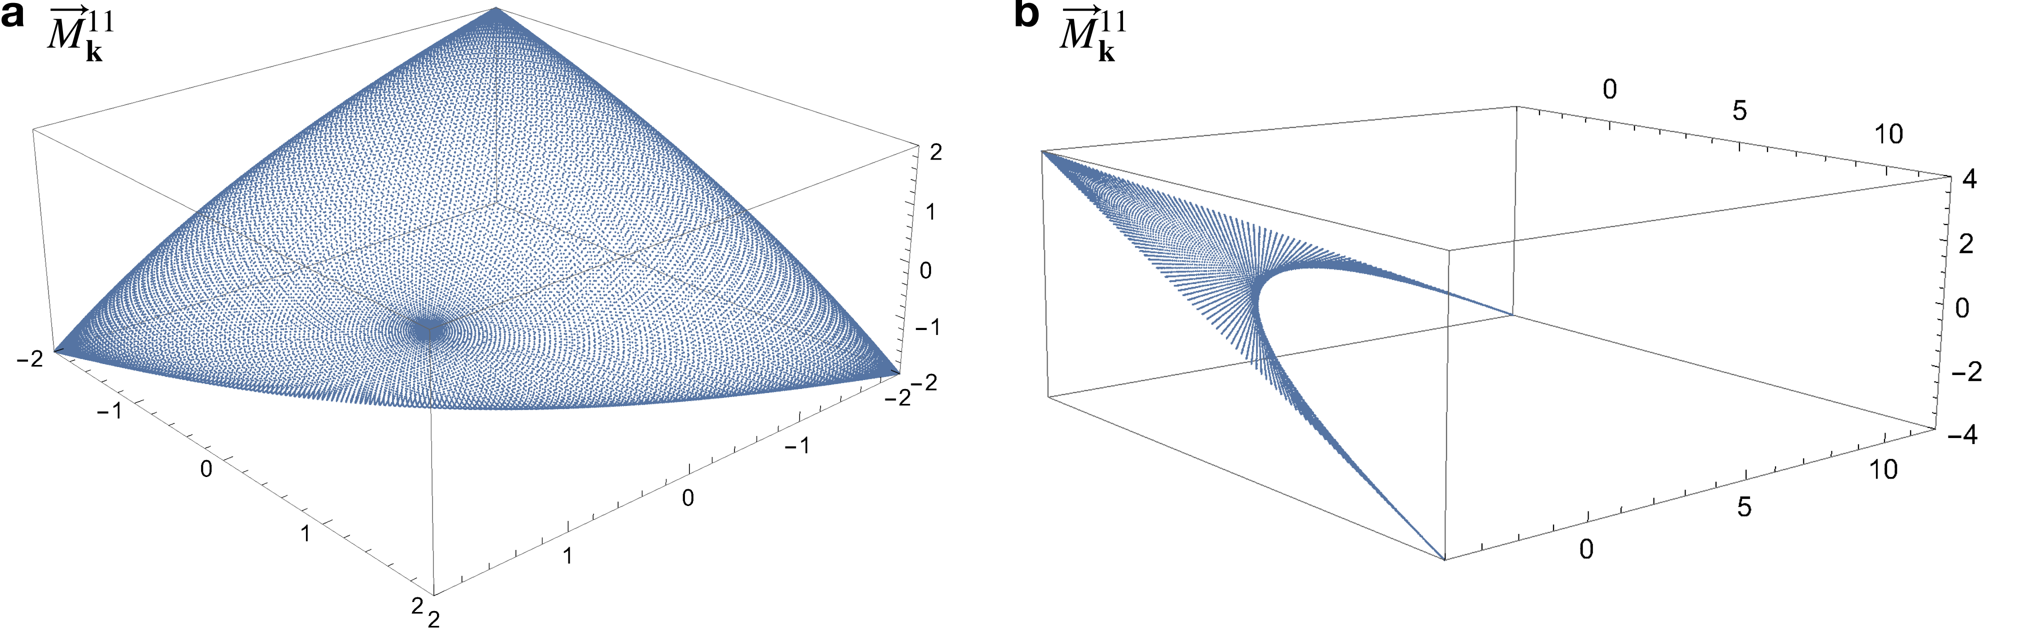
a
$\overrightarrow{M}_{\mathbf{k}}^{11}$
b
$\overrightarrow{M}_{\mathbf{k}}^{11}$
−2 −1 0 1 2
2 1 0 −1 −2
−2 −1 0 1 2
0 5 10
4 2 0 −2 −4
0 5 10

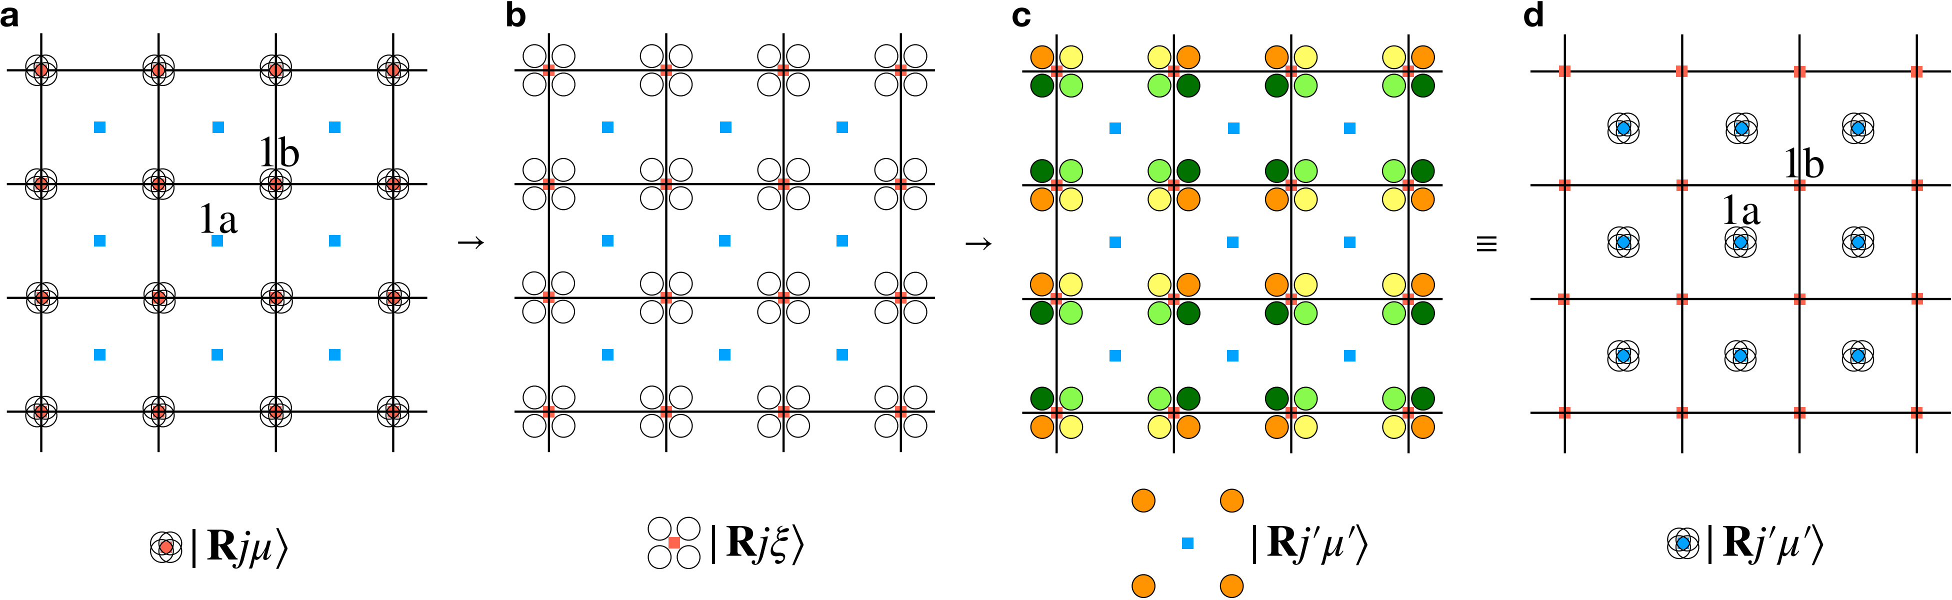
a
b
c
d
1b
1a
1b
1a
→
→
≡
$|\mathbf{R}j\mu\rangle$
$|\mathbf{R}j\xi\rangle$
$|\mathbf{R}j'\mu'\rangle$
$|\mathbf{R}j'\mu'\rangle$

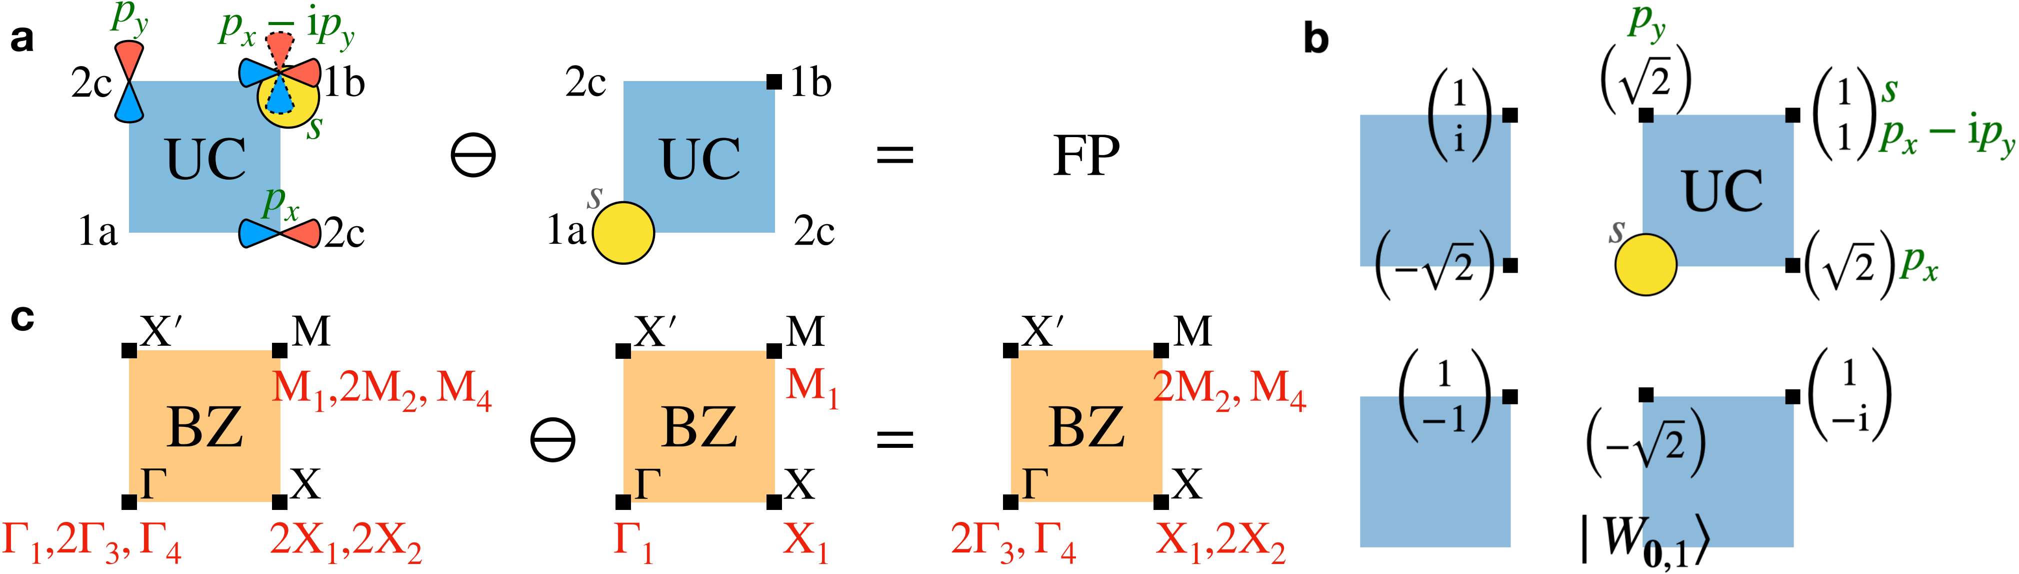
a
$p_y$
$p_x - \mathrm{i}p_y$
2c
1b
$s$
UC
$p_x$
1a
2c
⊖
2c
1b
UC
$s$
1a
2c
=
FP
b
$p_y$
$(\sqrt{2})$
$\begin{pmatrix}1\\ \mathrm{i}\end{pmatrix}$
$\begin{pmatrix}1\\ 1\end{pmatrix}$
$s$
$p_x - \mathrm{i}p_y$
UC
$(-\sqrt{2})$
$s$
$(\sqrt{2})$
$p_x$
$\begin{pmatrix}1\\ -1\end{pmatrix}$
$\begin{pmatrix}1\\ -\mathrm{i}\end{pmatrix}$
$(-\sqrt{2})$
$|W_{\mathbf{0},1}\rangle$
c
X′
M
BZ
Γ
X
$M_1, 2M_2, M_4$
$\Gamma_1, 2\Gamma_3, \Gamma_4$
$2X_1, 2X_2$
⊖
X′
M
BZ
Γ
X
$M_1$
$\Gamma_1$
$X_1$
=
X′
M
BZ
Γ
X
$2M_2, M_4$
$2\Gamma_3, \Gamma_4$
$X_1, 2X_2$

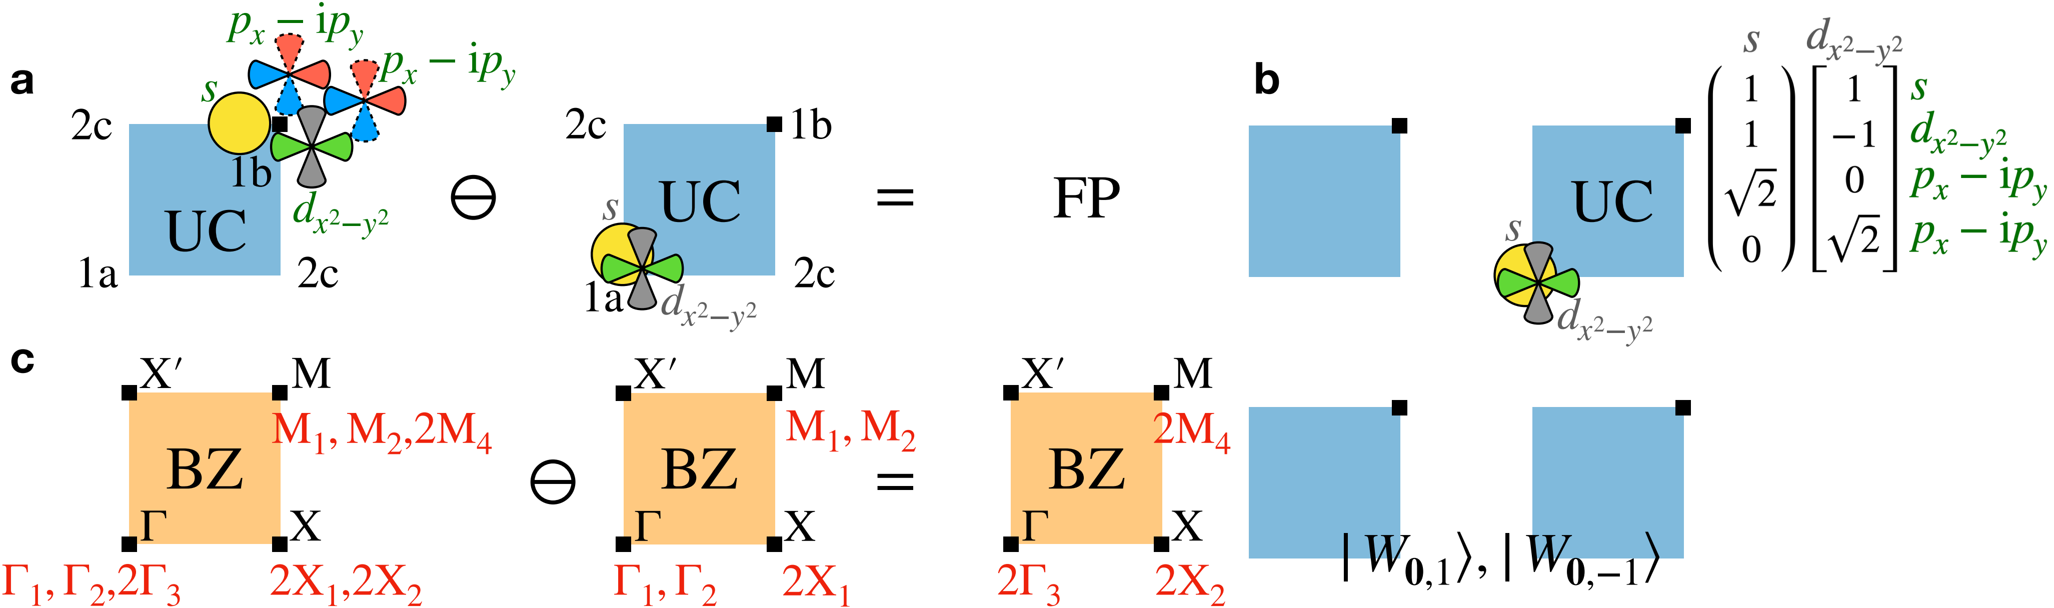
a
b
c
UC
FP
BZ
1a
1b
2c
s
$d_{x^2-y^2}$
$p_x - ip_y$
$\ominus$
=
$X'$
M
Γ
X
$M_1, M_2, 2M_4$
$\Gamma_1, \Gamma_2, 2\Gamma_3$
$2X_1, 2X_2$
$M_1, M_2$
$\Gamma_1, \Gamma_2$
$2X_1$
$2M_4$
$2\Gamma_3$
$2X_2$
$|W_{\mathbf{0},1}\rangle, |W_{\mathbf{0},-1}\rangle$

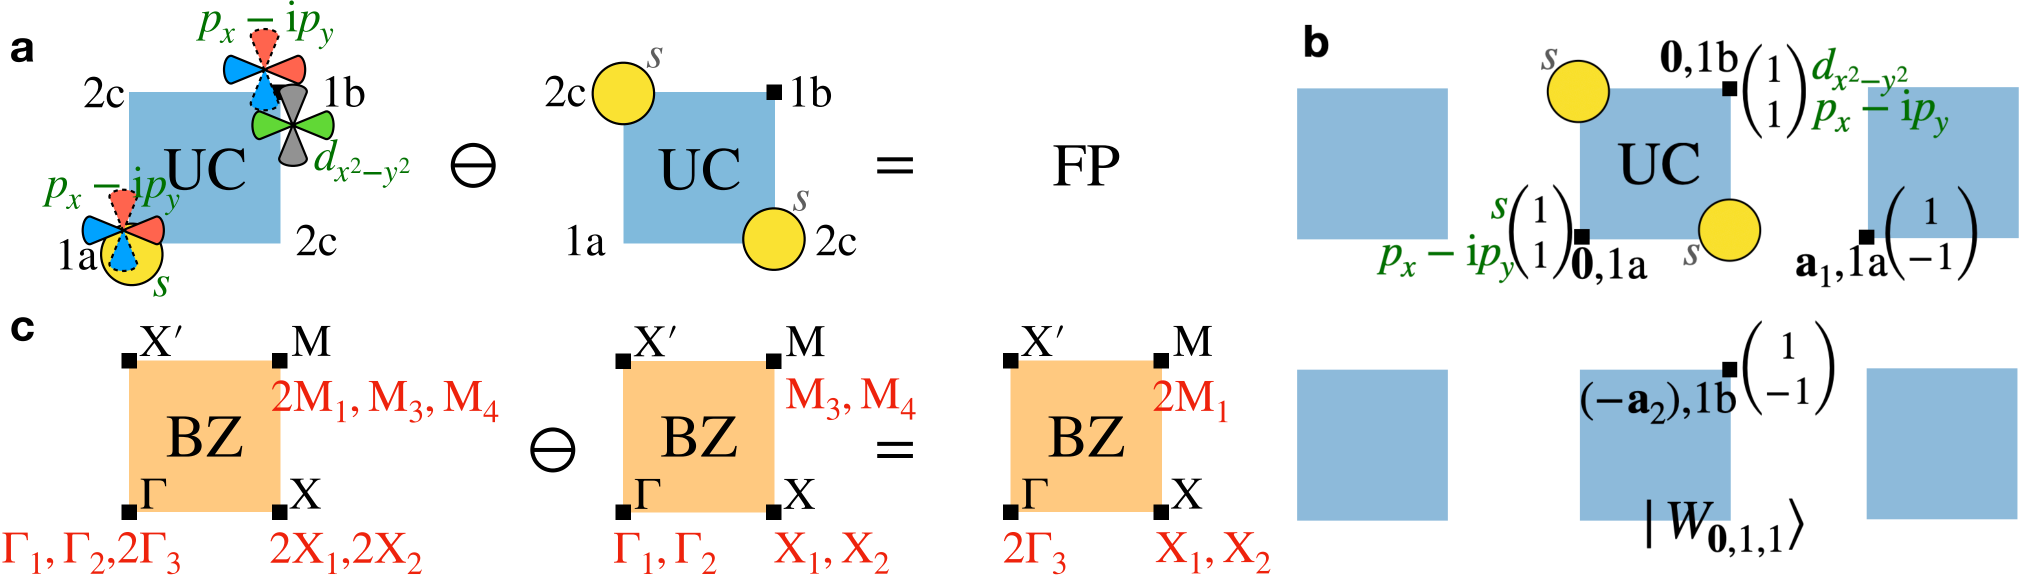
a
$p_x - ip_y$
2c
1b
UC
$d_{x^2-y^2}$
$p_x - ip_y$
1a
$s$
2c
⊖
$s$
2c
1b
UC
$s$
1a
2c
=
FP
b
$s$
$\mathbf{0}$,1b
$\begin{pmatrix}1\\1\end{pmatrix}$
$d_{x^2-y^2}$
$p_x - ip_y$
UC
$s$ $\begin{pmatrix}1\\1\end{pmatrix}$
$p_x - ip_y$
$\mathbf{0}$,1a
$s$
$\mathbf{a}_1$,1a $\begin{pmatrix}1\\-1\end{pmatrix}$
$(-\mathbf{a}_2)$,1b $\begin{pmatrix}1\\-1\end{pmatrix}$
$|W_{\mathbf{0},1,1}\rangle$
c
X′
M
BZ
$2M_1, M_3, M_4$
Γ
X
$\Gamma_1, \Gamma_2, 2\Gamma_3$
$2X_1, 2X_2$
⊖
X′
M
BZ
$M_3, M_4$
Γ
X
$\Gamma_1, \Gamma_2$
$X_1, X_2$
=
X′
M
BZ
$2M_1$
Γ
X
$2\Gamma_3$
$X_1, X_2$

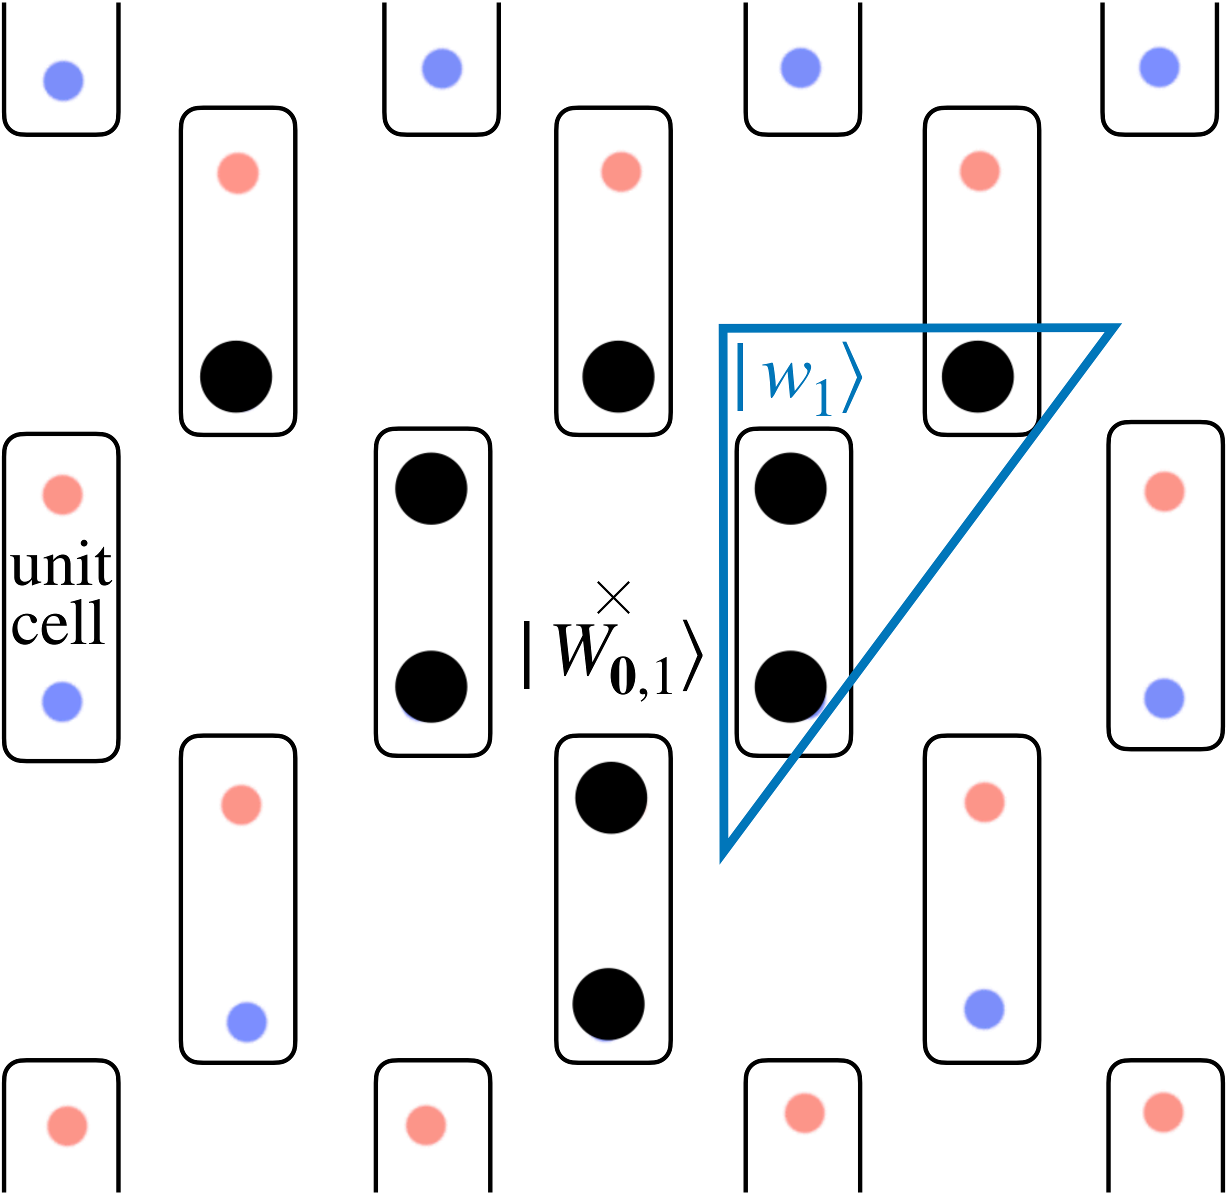

unit cell
$|\overset{\times}{W}_{\mathbf{0},1}\rangle$
$|w_1\rangle$

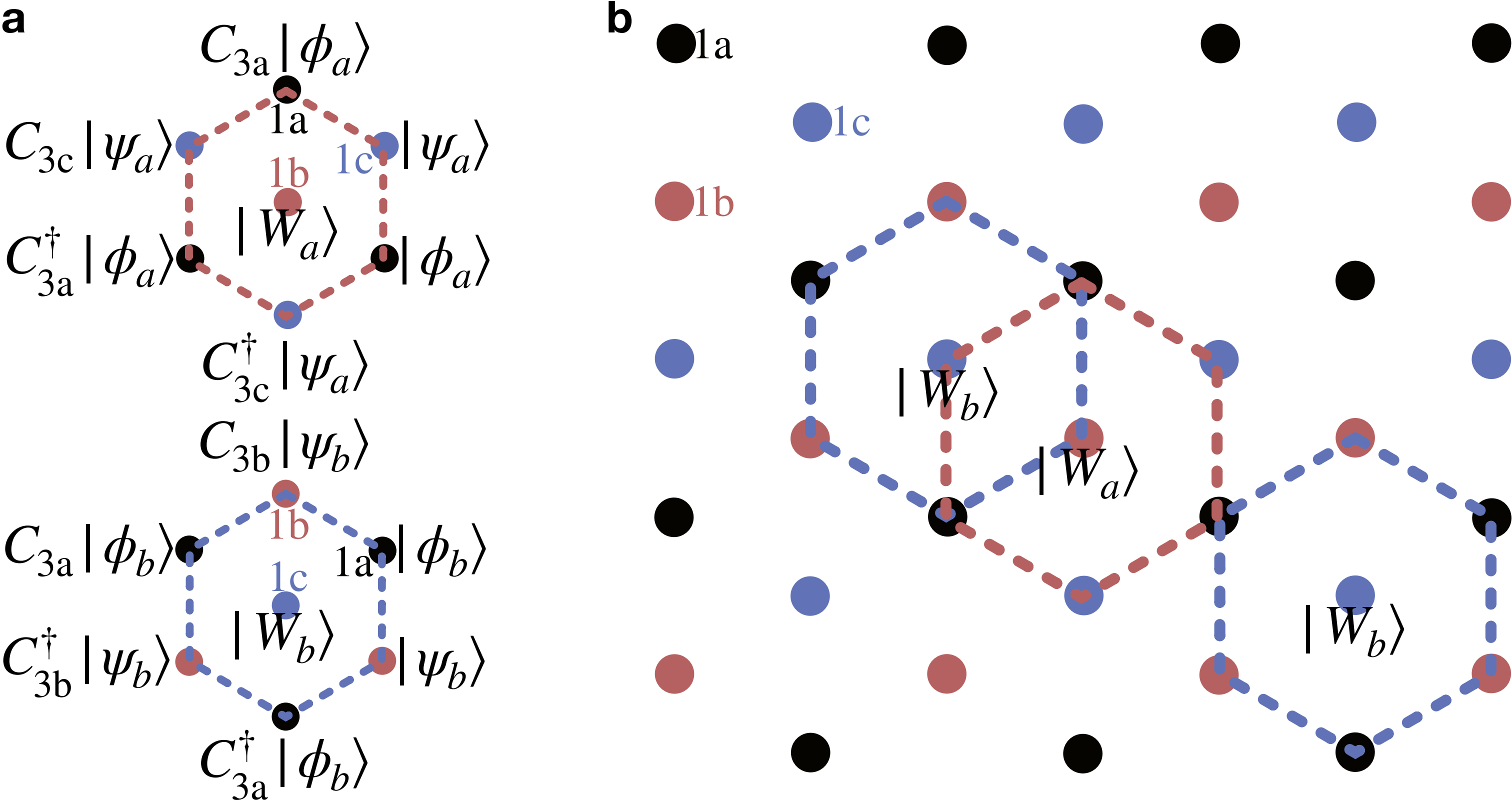
a
$C_{3a}|\phi_a\rangle$
1a
$C_{3c}|\psi_a\rangle$
$|\psi_a\rangle$
1b
1c
$|W_a\rangle$
$C^\dagger_{3a}|\phi_a\rangle$
$|\phi_a\rangle$
$C^\dagger_{3c}|\psi_a\rangle$
$C_{3b}|\psi_b\rangle$
1b
$C_{3a}|\phi_b\rangle$
$|\phi_b\rangle$
1a
1c
$|W_b\rangle$
$C^\dagger_{3b}|\psi_b\rangle$
$|\psi_b\rangle$
$C^\dagger_{3a}|\phi_b\rangle$
b
1a
1c
1b
$|W_b\rangle$
$|W_a\rangle$
$|W_b\rangle$

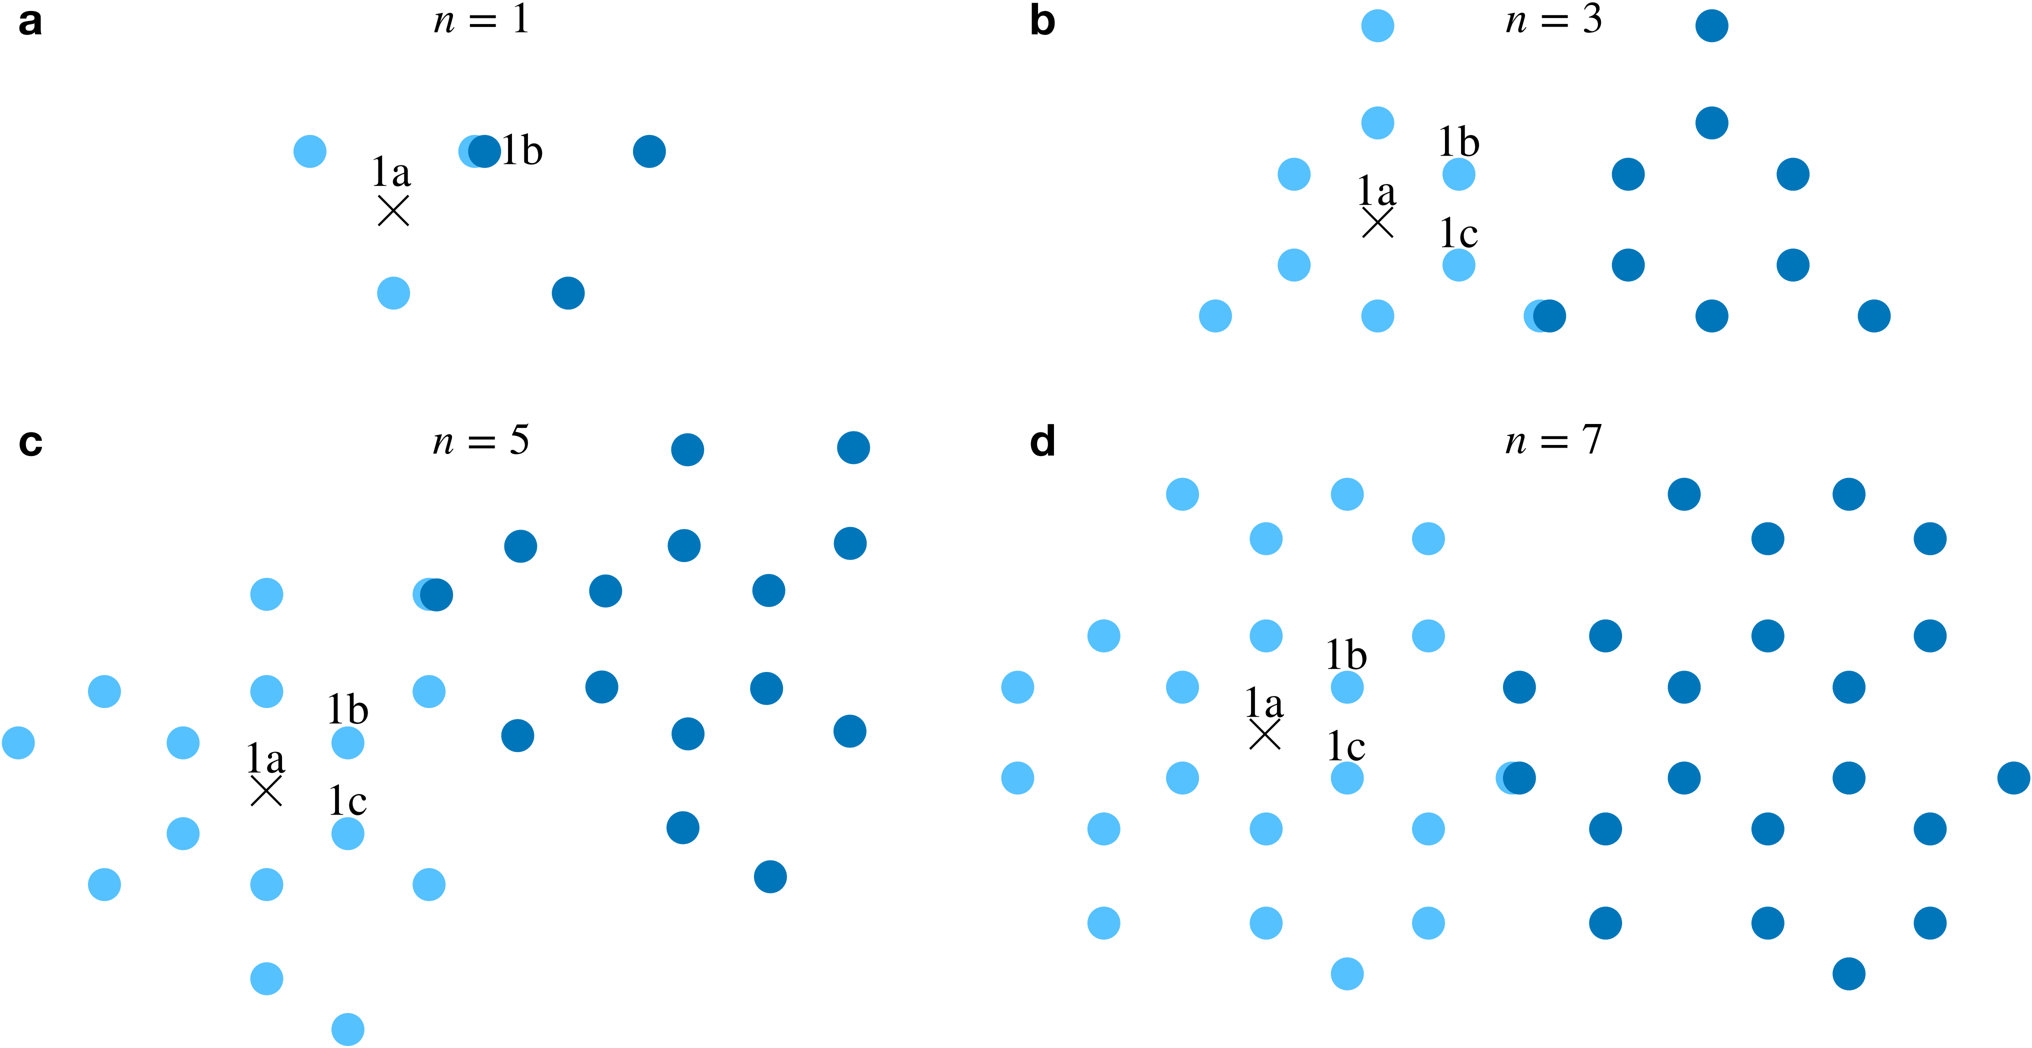
a
n = 1
1a
1b
b
n = 3
1a
1b
1c
c
n = 5
1a
1b
1c
d
n = 7
1a
1b
1c
